# Supplementary material for: Towards Effective Counter-Responses: Aligning Human Preferences with Strategies to Combat Online Trolling
Source: arXiv:2410.04164 source file (2024-10-05)
Supplement: Supplementary file 1 [file dataset_detail_statistics.tex]

\begin{table}[t!]
    \centering
    \resizebox{\columnwidth}{!}{
            \begin{tabular}{l|cc}
            \hline
            Category & Subreddits & Total \\
            \hline
            Discussion & Tech, Other & 222 \\
            Hobbies and Own & tt & 249 \\
            Lifestyle & r/teenager (13), & 249 \\
            \hline
        \end{tabular}
    }
    \caption{Data statistics}
    \label{tab:dataset_detail_statistics}
\end{table}
